# Supplementary material for: Transferability Through Cooperative Competitions
Source: arXiv:2603.27770 source file (2026-03-29)
Supplement: Supplementary file 1 [file appendix.tex]

\appendix
%%%%%%%%%%%%%%%%%%%%%%%%%%%%%%%%%%%%%%%%%%%%%%%%%%%%%%%%%%%%%%%%%%%%%%%%%%%%%%%%%%%%%
\begin{table*}[b]
\centering
%\vspace{10pt}  % Adds vertical space between "Table 1" and the table
\begin{minipage}{0.45\textwidth}
    \begin{tabular}{|c|c|c|}
    \hline
    \rowcolor[HTML]{cc7d7a}
    \textbf{Milestone} & \textbf{Task Description} & \textbf{Score} \\ \hline
    MS\textsubscript{1} & Press the blue button & 100 \\ \hline
    MS\textsubscript{2} & Pick up probe plug & 100 \\ \hline
    MS\textsubscript{3} & Insert probe plug & 300 \\ \hline
    MS\textsubscript{4} & Reach SP1 center on screen & 100 \\ \hline
    MS\textsubscript{5} & Reach SP2 on screen & 300 \\ \hline
    MS\textsubscript{6} & Open door & 200 \\ \hline
    MS\textsubscript{7} & Insert probe and close circuit & 400 \\ \hline
    MS\textsubscript{8} & Wrap cable & 400 \\ \hline
    MS\textsubscript{9} & Insert probe tip into holder & 100 \\ \hline
    MS\textsubscript{10} & Press the red button & 100 \\ \hline
    \end{tabular}
    %\caption{Milestones and scores in the Task Board Manipulation Challenge.}
    \label{tab:irl_milestones_scores}
\end{minipage}
\hfill
\begin{minipage}{0.45\textwidth}
    \begin{tabular}{|m{6cm}|m{0.4cm}|}
    \hline
    \rowcolor[HTML]{cc7d7a}
    \textbf{Milestone Conditional Level Description} & \textbf{$l_{m}$} \\ \hline
    The robot requires human assistance & 0.0 \\ \hline
    The robot is teleoperated within the operator’s line of sight & 0.3 \\ \hline
    Slider not actively perceived & 0.5 \\ \hline
    Cable partially wrapped (only a single loop around the supports) & 0.5 \\ \hline
    The robot is teleoperated from a remote location & 0.6 \\ \hline
    The team attaches a custom handle to the task board to accommodate their specific gripper & 0.6 \\ \hline
    The robot manipulator is fully autonomous and the task board is left unchanged & 1.0 \\ \hline
    \end{tabular}
    %\caption{Milestones conditional levels in the Task Board Manipulation Challenge.}
    \label{tab:irl_milestones_lm}
\end{minipage}

\vspace{10pt}

\begin{minipage}{0.45\textwidth}
    \begin{tabular}{|m{6cm}|m{0.4cm}|}
    \hline
    \rowcolor[HTML]{cc7d7a}
    \textbf{Milestone Penalties Description} & \textbf{$p_{m}$} \\ \hline
    The robot collides with the task board, table or any other object present in the environment & 100 \\ \hline
    \end{tabular}
    %\caption{Milestone penalties in the Task Board Manipulation Challenge.}
    \label{tab:irl_milestones_penalties}
\end{minipage}
\hfill
\begin{minipage}{0.45\textwidth}
    \begin{tabular}{|m{6cm}|m{0.4cm}|}
    \hline
    \rowcolor[HTML]{d8a69e}
    \textbf{Task Conditional Level Description} & \textbf{$T$} \\ \hline
    Task board fixed within the table & 0.6 \\ \hline
    Task board randomly positioned within the table & 1.0 \\ \hline
    \end{tabular}
    %\caption{Task conditional levels in the Task Board Manipulation Challenge.}
    \label{tab:irl_task_conditional_levels}
\end{minipage}
%\vspace{10pt}  % Adds vertical space between "Table 1" and the table
%\caption{Overview of milestones, conditional levels, penalties, and task conditional levels in the Task Board Manipulation Challenge.}
\label{tab:irl_scores_combined}
\end{table*}

%%%%%%%%%%%%%%%%%%%%%%%%%%%%%%%%%%%%%%%%%%%%%%%%%%%%%%%%%%%%%%%%%%%%%%%%%%%%%%%%%%%%%%%%%%
\begin{table*}[hb]
\centering
%\vspace{10pt}

% --- First Table (Milestones and Scores) ---
\begin{tabular}{|m{1.2cm}|m{3cm}|m{8.5cm}|m{.6cm}|}
\hline
\rowcolor[HTML]{4FAD6F}
\textbf{Milestone} & \textbf{Milestone Type} & \textbf{Task Description} & \textbf{Score} \\ \hline
MS\textsubscript{1} & Navigation & The robot navigates to the Instruction Point & 100 \\ \hline
MS\textsubscript{2} & Command Understanding & The robot understands the given instruction (the robot needs to reproduce the command using speech or written logs) & 100 \\ \hline
MS\textsubscript{3} & Navigation & The robot navigates to Location $L_{i}$ in Kitchen $K_{i}$ & 100 \\ \hline
MS\textsubscript{4} & Manipulation & The robot opens the door on his way to Kitchen $K_{i}$ (if required) & 400 \\ \hline
MS\textsubscript{5} & Manipulation & The robot opens the drawer/cabinet/dishwasher at Location $L_{i}$ in Kitchen $K_{i}$ (if required) & 200 \\ \hline
MS\textsubscript{6} & Object Detection & The robot detects the Object $O_{i}$ at Location $L_{i}$ in Kitchen $K_{i}$ & 100 \\ \hline
MS\textsubscript{7} & Manipulation & The robot picks the Object $O_{i}$ at Location $L_{i}$ in Kitchen $K_{i}$ & 400 \\ \hline
MS\textsubscript{8} & Navigation & The robot navigates to Location $L_{j}$ in Kitchen $K_{j}$ while carrying the object & 100 \\ \hline
MS\textsubscript{9} & Manipulation & The robot opens the door on his way to Kitchen $K_{j}$ while carrying the object (if required) & 600 \\ \hline
MS\textsubscript{10} & Manipulation & The robot places the Object $O_{i}$ at Location $L_{j}$ in Kitchen $K_{j}$ & 400 \\ \hline
MS\textsubscript{10} & Manipulation & The robot hands over the Object $O_{i}$ to Person $P_{i}$ in Kitchen $K_{j}$ & 600 \\ \hline
\end{tabular}

\vspace{1cm}  % Spacing between stacked tables

% --- Second Table (Milestone Conditional Levels) ---
\begin{tabular}{|m{3cm}|m{10.5cm}|m{0.4cm}|}
\hline
\rowcolor[HTML]{4FAD6F}
\textbf{Milestone type} & \textbf{Milestone Conditional Level Description} & \textbf{$l_{m}$} \\ \hline
\multirow{4}{1.8cm}{Navigation} & The robot is teleoperated within the operator’s line of sight & 0.3 \\ \cline{2-3} 
& The robot is teleoperated from a remote location & 0.6 \\ \cline{2-3} 
& The robot uses artificial landmarks (i.e. aruco markers or april tags) to localize & 0.6 \\ \cline{2-3} 
& The robot is fully autonomous. No teleoperation or artificial landmarks & 1.0 \\ \hline
\multirow{3}{1.8cm}{Command Understanding} & The team runs script, i.e. bypass natural language understanding and speech-to-text & 0.0 \\ \cline{2-3}
& The command is given by command line or any other interface, i.e. bypass speech-to-text & 0.4 \\ \cline{2-3}
& The robot understands the command via speech & 1.0 \\ \hline
\multirow{5}{1.8cm}{Manipulation} & The robot requires human assistance & 0.0 \\ \cline{2-3}
& The robot is teleoperated within the operator’s line of sight & 0.3 \\ \cline{2-3}
& The robot is teleoperated from a remote location & 0.6 \\ \cline{2-3}
& The team attaches a custom handle to the object to accommodate their specific gripper & 0.6 \\ \cline{2-3}
& A standard unmodified handle is used for object manipulation & 1.0 \\ \hline
\multirow{3}{1.8cm}{Perception} & Only the target object is initially placed in Location $L_{i}$ & 0.4 \\ \cline{2-3}
& Several different objects are in Location $L_{i}$ without any occlusions from the robot’s POV (Known/Unknown Objects) & \makecell{0.6 \\ 0.8} \\ \cline{2-3}
& Several different objects are in Location $L_{i}$, and the target object to be picked up is either hidden behind another object or at least only partially visible (Known/Unknown Objects) & \makecell{0.8 \\ 1.0} \\ \hline
\end{tabular}

\vspace{1cm}

% --- Remaining two tables side by side ---
\begin{minipage}{0.45\textwidth}
    \begin{tabular}{|m{1.8cm}|m{5cm}|m{0.65cm}|}
    \hline
    \rowcolor[HTML]{4FAD6F}
    \textbf{Milestone type} & \textbf{Milestone Penalties Description} & \textbf{$p_{m}$} \\ \hline
    Navigation & The robot hits obstacles & 200 \\ \hline
    \multirow{2}{1.8cm}{Manipulation} & The robot collides with objects present in the environment & 200 \\ \cline{2-3}
    & The robot picks the wrong object & 200 \\ \hline
    Perception & The robot uses artificial landmarks & 50 \\ \hline
    \end{tabular}
\end{minipage}
\hfill
\begin{minipage}{0.45\textwidth}
    \begin{tabular}{|m{6cm}|m{0.4cm}|}
    \hline
    \rowcolor[HTML]{6ACF84}
    \textbf{Task Conditional Level Description} & \textbf{$T$} \\ \hline
    Task variables randomly generated ($L_{i}$, $L_{j}$, $O_{i}$) & 1.0 \\ \hline
    The teams specify one variable & 0.7 \\ \hline
    The teams specify two variables & 0.4 \\ \hline
    The teams specify all three variables & 0.3 \\ \hline
    \end{tabular}
\end{minipage}

%\vspace{10pt}
%\caption{Overview of milestones, conditional levels, penalties, and task conditional levels in the \textit{Multi-Functional Service Robot Challenge}.}
\label{tab:srl_scores_combined}
\end{table*}

%%%%%%%%%%%%%%%%%%%%%%%%%%%%%%%%%%%%%%%%%%%%%%%%%%%%%%%%%%%%%%%%%%%%%%%%%%%%%%%%%%%%%%%%%%

\begin{table*}[ht]
\centering
\vspace{10pt}

% --- First Table (Milestones and Scores) ---
\begin{tabular}{|m{1.2cm}|m{3cm}|m{8.5cm}|m{.6cm}|}
\hline
\rowcolor[HTML]{809FEF}
\textbf{Milestone} & \textbf{Milestone Type} & \textbf{Task Description} & \textbf{Score} \\ \hline
MS\textsubscript{1} & Navigation & The robot navigates to the Instruction Point & 100 \\ \hline
MS\textsubscript{2} & Command Understanding & The robot understands the given instruction (the robot needs to reproduce the command using speech or written logs) & 100 \\ \hline
MS\textsubscript{3} & Navigation & The robot navigates to Pick-Up Point $L_{i}$ to retrieve Parcel $O_{i}$ & 200 \\ \hline
MS\textsubscript{4} & Manipulation & The robot opens the door on his way to Pick-Up Point $L_{i}$ (if required) & 600 \\ \hline
MS\textsubscript{5} & Object Detection & The robot detects the Parcel $O_{i}$ at Pick-Up Point $L_{i}$ & 100 \\ \hline
MS\textsubscript{6} & Manipulation & The robot picks the Parcel $O_{i}$ from Pick-Up Point $L_{i}$ & 300 \\ \hline
MS\textsubscript{7} & Navigation & The robot navigates to Delivery Point $L_{j}$ while carrying the parcel & 200 \\ \hline
MS\textsubscript{8} & Manipulation & The robot opens the door on his way to Delivery Point $L_{j}$ while carrying the parcel (if required) & 600 \\ \hline
MS\textsubscript{9} & Manipulation & The robot drops the Parcel $O_{i}$ at Delivery Point $L_{j}$ & 200 \\ \hline
\end{tabular}

\vspace{1cm}  % Spacing between stacked tables

% --- Second Table (Milestone Conditional Levels) ---
\begin{tabular}{|m{3cm}|m{10.5cm}|m{0.4cm}|}
\hline
\rowcolor[HTML]{809FEF}
\textbf{Milestone type} & \textbf{Milestone Conditional Level Description} & \textbf{$l_{m}$} \\ \hline
\multirow{4}{1.8cm}{Navigation} & The robot is teleoperated within the operator’s line of sight & 0.3 \\ \cline{2-3} 
& The robot is teleoperated from a remote location & 0.6 \\ \cline{2-3} 
& The robot uses artificial landmarks (i.e. aruco markers or april tags) to localize & 0.6 \\ \cline{2-3} 
& The robot is fully autonomous. No teleoperation or artificial landmarks & 1.0 \\ \hline
\multirow{3}{1.8cm}{Command Understanding} & The team runs script, i.e. bypass natural language understanding and speech-to-text & 0.0 \\ \cline{2-3}
& The command is given by command line or any other interface, i.e. bypass speech-to-text & 0.4 \\ \cline{2-3}
& The robot understands the command via speech & 1.0 \\ \hline
\multirow{5}{1.8cm}{Manipulation} & The robot requires human assistance & 0.0 \\ \cline{2-3}
& The robot is teleoperated within the operator’s line of sight & 0.3 \\ \cline{2-3}
& The robot is teleoperated from a remote location & 0.6 \\ \cline{2-3}
& The team attaches a custom handle to the object to accommodate their specific gripper & 0.6 \\ \cline{2-3}
& A standard unmodified handle is used for object manipulation & 1.0 \\ \hline
\multirow{2}{1.8cm}{Perception} & Only the target Parcel $O_{i}$ is initially placed in the Pick-Up Point $L_{i}$ & 0.4 \\ \cline{2-3}
& Several different Parcels are in Pick-Up Point $L_{i}$ without any occlusions from the robot’s point-of-view & 1.0 \\ \hline
\end{tabular}

\vspace{1cm}

% --- Remaining two tables side by side ---
\begin{minipage}{0.5\textwidth}
    \begin{tabular}{|m{1.8cm}|m{4cm}|m{0.65cm}|}
    \hline
    \rowcolor[HTML]{809FEF}
    \textbf{Milestone type} & \textbf{Milestone Penalties Description} & \textbf{$p_{m}$} \\ \hline
    Navigation & The robot hits obstacles & 200 \\ \hline
    \multirow{2}{1.8cm}{Manipulation} & The robot collides with objects present in the environment & 200 \\ \cline{2-3}
    & The robot picks the wrong parcel & 200 \\ \hline
    Perception & The robot uses artificial landmarks & 50 \\ \hline
    \end{tabular}
\end{minipage}
\hfill
\begin{minipage}{0.47\textwidth}
    \begin{tabular}{|m{6cm}|m{0.4cm}|}
    \hline
    \rowcolor[HTML]{809FEF}
    \textbf{Task Conditional Level Description} & \textbf{$T$} \\ \hline
    Task variables randomly generated ($L_{i}$, $L_{j}$, $O_{i}$) & 1.0 \\ \hline
    The team specifies one variable & 0.7 \\ \hline
    The team specifies two variables & 0.4 \\ \hline
    The team specifies three variables & 0.3 \\ \hline
    \end{tabular}
\end{minipage}

\vspace{10pt}
\caption{Overview of milestones, conditional levels, penalties, and task conditional levels in the \textit{Delivery Robot Challenge}.}
\label{tab:orl_scores_combined}
\end{table*}
